# Supplementary material for: Neural Text Summarization: A Critical Evaluation
Source: arXiv:1908.08960 source file (2019-08-23)
Supplement: Supplementary file 1 [file appendix-background.tex]

\section{Neural models analyzed in this study}
% Describe models used for this study
\citet{Hsu:18} used a hybrid architecture combining an extractor with an abstractor.
The the role of the extractor was to return a sentence-level distribution over the source document that was used to scale the word-level attention distribution of the abstractor during decoding.
The authors added a penalty term to the training objective to penalize inconsistencies between the two levels of attention.

In \citet{Gehrmann:18} the authors combined a content selection model with and abstractive summarizaton model.
The content selector generated a word-level mask over the source documents that was used to guide the copy attention distribution of the abstractive summarizer during decoding.

\citet{Jiang:18} proposed a training strategy that improved the memorization and information selection capabilities of the encoder.
The authors augmented the attention-based encoder-decoder architecture with an additional decoder without access to attention of copying mechanisms.
The model was trained using the loss coming from both decoders simultaneously, forcing the encoder to create more information-rich hidden states to accommodate the limitations of the restricted decoder.

\citet{Chen:18} proposed using a two component, extractive and abstractive architecture trained using reinforcement learning techniques.
Generation was conducted in two phases: first, the extractive model selected sentences that would be used in the summary, then the abstractive model would paraphrase and compress those selections.
The model was trained in an end-to-end fashion using a policy-based training strategy.

\citet{See:17} proposed an encoder-decoder architecture with attention and copying mechanisms.
The architecture was augmented with a coverage mechanism that prevented the model from attending multiple times to the same spans of the source documents.
The coverage mechanism was used as a regularization term in the objective function.

In \citet{Kryscinski:18} the authors decomposed the decoder of a standard encoder-decoder architecture into two components: a language model and a contextual model. 
The architecture was trained using a hybrid loss, cross-entropy and policy gradients, with rewards coming from the ROUGE toolkit and a Novelty metric.

\citet{WLi:18} the authors augment an abstractive encoder-decoder architecture with an explicit layer for information selection.
The proposed architecture consisted of three layers: encoding layers, information selection layer, and decoding layer and was trained in an end-to-end fashion.

\citet{Pasunuru:18} proposed a multi-reward training strategy that incorporated rewards from an entailment model and the ROUGE metric.
The introduced model was encouraged during training to generate summaries with high logical entailment with the source document.

\citet{Zhang:18} used an standard encoder-decoder architecture with pointing mechanisms where the decoding was done solely by means on copying tokens via the copying mechanism.
The authors showed that such an approach achievs similar level of abstraction to fully abstractive models.

\citet{Guo:18} proposed training abstractive summarization models in a multi-task regime, where the auxiliary were natural language inference and question generation.
The proposed model had task-specific layers, but incorporated soft weight sharing in the lower-layers of both the encoder and decoder models.

\citet{Dong:18} \\
\citet{Wu:18} 

\citet{Zhao:18} proposed an end-to-end extractive architecture for scoring and selecting sentences from the source document.
The model used a hierarchical encoder to build an information-rich representation of the source document and next jointly scored and selected the fragments to be included in the summary.
