# Supplementary material for: Neural Text Summarization: A Critical Evaluation
Source: arXiv:1908.08960 source file (2019-08-23)
Supplement: Supplementary file 2 [file appendix-examples.tex]

\section{Additional Experiment Examples}
All examples in the following sections were randomly sampled and are representative of the underlying problem.
% TABLE USED TO BE HERE.
\begin{table*}[t]
    \begin{center}
        \resizebox{\linewidth}{!}{%
        \small
        \begin{tabular}{p{0.49\linewidth}|p{0.49\linewidth}} 
        \toprule
        \textit{Article A} & \textit{Article B} \\ 
        \midrule
        babies born on the same day as the royal baby will be eligible to receive one of 2,015 free `lucky 'silver pennies. the royal mint announced it will \textcolor{blue}{mark the birth of the duke and duchess of cambridge's second child in the same way it commemorated the arrival of prince george in 2013}. parents of newborns who share a birthday with the new prince or princess, due later this month, will have to register the birth of their child on the royal mint's facebook page to receive the commemorative gift. (...) & 
        first impressions are not necessarily the best. when adam lyth scratched around for 22 in a championship match against nottinghamshire in 2008, graeme swann branded him a `walking wicket '.` but then,' swann added. `he proved us all wrong. 'lyth, one of six yorkshire players in the england squad that left heathrow on thursday for three tests in the caribbean, hit back in that match seven years ago with a second-innings of 132. wisden later called him` the find of the season'. yorkshire's adam lyth fields during day three of the champion county match against the mcc. \textcolor{blue}{now he finds himself competing with jonathan trott to be alastair cook's opening partner at the first test in antigua on april 13}. it has been quite a rise. (...) \\ 
        \midrule
        \textit{Summary A - Temporal inaccuracy} & 
        \textit{Summary B - Other inaccuracy} \\ 
        \midrule
        babies born on same day as royal baby will be eligible to receive one of 2,015 free `lucky 'silver pennies. royal mint will \textcolor{red}{mark the birth of the duke and duchess of cambridge's second child in 2013}. parents of newborns will have to register the birth of their child. (...) & 
        adam lyth, one of six yorkshire players in the championship match against nottinghamshire in 2008. graeme swann branded him a `walking wicket 'and` it's just about the moon'. he said he `proved us all wrong '. \textcolor{red}{lyth, 22, is a alastair cook's opening partner at antigua on april 13}. \\
        \midrule
        \textit{Article C} & \textit{Article D} \\ 
        \midrule
        cole skuse's first ipswich town goal, in their win against cardiff city which kept them in the final playoff spot, was a long time coming but boy was it worth the wait. \textcolor{blue}{after 21 months and 82 appearances since he signed from bristol city in july 2013, skuse opened his account with a 30-yard effort which could barely have been struck sweeter}. (...) &
        britain's aid budget may have to soar by hundreds of millions of pounds a year because of new eu rules, it has emerged. despite the fact that the uk has now met the controversial target to spend \textcolor{red}{0.7 per cent of national income on overseas aid}, changes to brussels accounting rules could bump up the bill even more. (...) \\
        \midrule
        \textit{Summary C - Temporal inaccuracy} & 
        \textit{Summary D - Numerical inaccuracy} \\ 
        \midrule
        \textcolor{red}{cole skuse opened his scoring for ipswich in july 2013}. bruno ecuele manga scored the only goal goal in the win. cardiff beat cardiff city in the final round on the 90th minute. (...) &
        \textcolor{red}{7 per cent of national income on overseas aid}, changes to brussels accounting rules could bump up the bill even more. 7\% of foreign aid, 7\%, spending \# 11. (...) \\
        \bottomrule
        \end{tabular}
        }%
    \caption{Examples of four news articles with factually incorrect summaries generated by abstractive models.}
    \label{tab:app-factual-errors}
    \end{center}
\end{table*}

\begin{table*}[t]
    \begin{center}
    \resizebox{\linewidth}{!}{%
    \small
        \begin{tabular}{p{0.49\linewidth}p{0.49\linewidth}} 
        \toprule
        \textit{CNN/DM - Links to other articles} &
        \textit{CNN/DM - Links to other articles} \\ 
        \midrule
        Aston Villa owner Randy Lerner in discussions to sell the club. 
        Manager Tim Sherwood not concerned by takeover talks. 
        Sherwood says he is focused on survival and building for next season. 
        Aston Villa are 16th and three points clear of relegation zone.
        \textcolor{red}{CLICK HERE for the latest Aston Villa news.} & 
        PSG travel to Nou Camp on Tuesday with Barcelona in command of the tie. 
        Luis Suarez inspired Barca to 3-1 win in Paris. 
        But Zlatan Ibrahimovic will return for second leg in Spain. 
        Blanc says Barca have `incredible talent' but his side have nothing to lose. 
        \textcolor{red}{READ: Egotistic Ibrahimovic will believe Barcelona will be in awe of him.} \\
        \toprule
        \textit{Newsroom - Non informative summary} &
        \textit{Newsroom - Unparsed HTML} \\ 
        \midrule
        \textcolor{red}{By Jim Dalrymple, Austin} &
        \textcolor{red}{New York Post Online: Sports: New York Islanders><meta name=} \\
        \bottomrule
        \end{tabular}
    }%
    \caption{
    Examples of noisy reference summaries found in the CNN/DM and Newsroom datasets.
    }
    \label{tab:noisy-labels}
    \end{center}
\end{table*}
